# Supplementary material for: Fast Empirical Scenarios
Source: arXiv:2307.03927 source file (2024-11-05)
Supplement: Supplementary file 1 [file revised_appendix.tex]

\begin{comment}
\appendix
\section{Notations}\label{appendix:notations}
For this section, we  introduce the following notations,
\begin{enumerate}
    \item $\big(\Cscr(\Xcal), \|\cdot\|_{\infty}\big)$: the Banach space of continuous real-valued functions on $\Xcal$, equipped with the supremum norm,
    \item $\big(\Cscr_{b}(\Xcal), \|\cdot\|_{\infty}\big)$: the Banach space of bounded continuous real-valued functions on $\Xcal$, equipped with the supremum norm,
    \item $\big(\Mscr(\Xcal), |\cdot|\big):$ the Banach space of finite signed Borel measures on $\Xcal$, equipped with the total variation norm,
    \item $\Mscr_{+}^{1}(\Xcal)$: the set of probability measures on $\Xcal$, that is a convex subset of $\Mscr(\Xcal)$.
\end{enumerate}
We now provide a short remark regarding Problem \ref{eq:relaxedmm}.
\begin{remark}\label{rem:problem_formulation}
    From \cite[Theorem 14.15]{InfiniteDimensionalAnalysis}, we know that for a compact metrizable space $X$, $\Cscr(X)^\ast$ can be identified with $\Mscr(X)$, which now contains just finite Borel measures on $X$, and $\Mscr(X) \supset \Mscr^1_{+}(X)$. However, we cannot characterize $\Mscr^1_{+}(X)$ as the dual of any space and hence using the (dual) total variation norm to measure the \enquote{closeness} of $\Pbb^\star, \widehat\Pbb$ becomes too restrictive. So we resort to \cite[Theorem 15.1]{InfiniteDimensionalAnalysis} to have a weaker notion of the closeness; we know that any $\Pbb \in \Mscr_{+}^{1}(X)$ gives rise to a unique linear mapping $f \mapsto \int f\d\Pbb$ from  ${\Cscr_{b}(X)} = {\Cscr(X)}$ (since $X$ is compact) to $\Rbb$. Hence, we can say $\Pbb^\star, \widehat\Pbb \in \Mscr_{+}^{1}(X)$ are close in the weak-* sense if $\int f \d\Pbb^\star = \int f\d\widehat\Pbb$ for all $f \in \Cscr(X)$. Again, from the Stone-Weierstrass theorem, we have that the algebra of all polynomials $\cup_{q \in \N} \Pscr_{q}(X)$ is dense in $\Cscr(X)$. However, for moment-matching up to total degree $2q$ (with $q$ fixed), we restrict our attention to $\Pscr_{2q}(X)$. To speak loosely, we expect the compressed measure $\Pbb^\star$ to \enquote{be close} to $\widehat{\Pbb}$ (in the sense of weak-* topology) if we test their expectations on $\Pscr_{2q}(X)$ i.e.\,solve Problem \eqref{eq:relaxedmm}. Furthermore, since on finite-dimensional normed spaces, all norms are equivalent, herein we do not consider the supremum norm on $\Pscr_{2q}(X)$ (which translates to the worst-case error) and instead choose the Euclidean norm, that can be interpreted as the mean-squared error.
\end{remark}

\section{Lasserre's algorithm}\label{appendix:lasserre} To make the paper
self-contained, we  include  here a method to find flat
extension of input moment matrices and Lasserre's algorithm for
scenario extraction cp. \cite[Chapter 4.3]{Lasserre} with a
modification for handling the rank-deficient case as well.
\subsection{Finding flat extensions}
Theorem \ref{res:curtofialkow} reveals that 
the computation of scenarios can be performed via the flat extension
of the moment matrix. Except for specialized cases, when the moment
matrix is singular or the associated variety is finite, etc., for
the general case when the moment matrix is positive definite,
methods to find flat extensions are relatively unexplored.
We propose
here a method that involves solving a sequence of trace
minimization problems for finding flat extensions through
semidefinite programming (SDP). We start from a rank-$r$ input
moment matrix $\boldsymbol M _{\boldsymbol y}\in
\Rbb ^{m_q\times m_q}$ with the goal to find its flat extension
$\boldsymbol M _{\tilde{\boldsymbol y}}\in \Rbb^{m_{q+l}\times
m_{q+l}}$ for some $l\geq 1$. Introducing the block matrix representation 
\begin{equation*}
\boldsymbol M _{\tilde{\boldsymbol y}}=\begin{bmatrix}
\boldsymbol A _{\tilde{\boldsymbol y}} &
\boldsymbol B_{\tilde{\boldsymbol y}} \\  
\boldsymbol B_{\tilde{\boldsymbol y}}^{\top} &
\boldsymbol C_{\tilde{\boldsymbol y}}
\end{bmatrix}
\end{equation*}
with
\[
{\boldsymbol A _{\tilde y}\in\Rbb^{m_{q+l-1}\times m_{q+l-1}}},\
                  {\boldsymbol B_{\tilde y}\in\Rbb^{m_{q+l-1}
                  \times (m_{q+l}-m_{q+l-1})}},\
                  {\boldsymbol C_{\tilde y}\in\Rbb^{(m_{q+l}-
                  m_{q+l-1})\times (m_{q+l}-m_{q+l-1})}}.
\]
Clearly there holds $\boldsymbol A _{\tilde{\boldsymbol y}}
=\boldsymbol M_{\boldsymbol y}$ if $\tilde y_{\boldsymbol\alpha}
=y_{\boldsymbol\alpha}$
for \(|\boldsymbol\alpha|\leq q\). We subsequently solve a convex
relaxation of the rank minimization problem by minimizing the
trace of the bottom-right block.

\begin{algorithm}\caption{SDP Flat Extension}
\begin{enumerate}
 \item Initialize $k\isdef 1$
 \item 
 \begin{align*}
  \underset{\tilde{\boldsymbol y}\in \Rbb^{m_{2(q+k)}}}{\text{ minimize }} & \trace(\boldsymbol C _{\tilde {\boldsymbol y}}) \\
  \text{subject to } & \tilde y_{\boldsymbol \alpha}=y_{\boldsymbol \alpha}, \, |\boldsymbol \alpha| \leq m_q\\
  & \boldsymbol M_{\tilde {\boldsymbol y}} \geq \boldsymbol 0
 \end{align*}
\item If $\rank \boldsymbol M_{\tilde {\boldsymbol y}} \leq  r$ terminate, otherwise increment $k\isdef k+1$ and return to (2)
\end{enumerate}
\end{algorithm}
However, there is no guarantee that this algorithm converges after a finite number of steps.
Furthermore, the size of the SDP grows exponentially fast with $k$, and the termination criterion of the algorithm necessitates the numerical  computation
of $\rank \boldsymbol M_{\tilde {\boldsymbol y}}$, as described below in Algorithm  \ref{algo:pivChol_flat}.

\subsection{Lasserre's extraction algorithm specialized to pivoted Cholesky decomposition}\label{sec:lasserrealgo}
Given a flat extension ${\boldsymbol M}_{\tilde{\boldsymbol y}}$ of
${\boldsymbol M}_{{\boldsymbol y}}$, we consider a modified version of 
the extraction algorithm suggested in \cite{Lasserre}. To handle the rank deficiency of the input moment matrix, we start from the pivoted Cholesky decomposition, cp.\ \cite{HPS12},
of ${\boldsymbol M}_{\tilde{\boldsymbol y}}$.
\begin{algorithm}\caption{Pivoted Cholesky decomposition (specialization to flat extensions)}
\label{algo:pivChol_flat}
\begin{flushleft}
\begin{tabular}{ll}
\textbf{input:}  & symmetric and positive semi-definite moment matrix ${\boldsymbol M}\in\mathbb{R}^{m_{q+l}\times m_{q+l}}$\\  
& tolerance \(\varepsilon>0\)\\
\textbf{output:} & low-rank approximation 
\({\boldsymbol M}\approx{\boldsymbol L}{\boldsymbol L}^\top\)
\end{tabular}
\end{flushleft}
%=================================================================================
\begin{algorithmic}[1]
\State Initialization: set $m\isdef 1$,
 ${\boldsymbol d}\isdef \operatorname{diag}({\boldsymbol M
})$, \({\boldsymbol L}\isdef[\,]\),
$\operatorname{err}\isdef \|{\boldsymbol d}\|_{1}$
\State\textbf{while} \(\operatorname{err}>\varepsilon\)
\State\StateIndent determine
$j\isdef \operatorname{arg}\max_{1\le i\le m_{q+\ell-1}} d_i$
\State\StateIndent compute \[\boldsymbol\ell_m
\isdef \frac{1}{\sqrt{d_j}}\Big({\boldsymbol M}-{\boldsymbol L}{\boldsymbol L}^\top\Big)\boldsymbol e_j
\]
\State\StateIndent set \({\boldsymbol L}
\isdef [{\boldsymbol L},\, {\boldsymbol\ell}_m]\),
\State\StateIndent set \({\boldsymbol d}\isdef {\boldsymbol d}-{\boldsymbol\ell}_m\odot
\,{\boldsymbol\ell}_m\), where $\odot$ denotes the Hadamard product
\State\StateIndent set \(\operatorname{err}\isdef\|{\boldsymbol d}\|_1\)
\State\StateIndent set \(m\isdef m+1\)
\end{algorithmic}
\end{algorithm}
Through the permutation matrix \({\boldsymbol P}\) determined from the pivot selection in line 3 of Algorithm~\ref{algo:pivChol_flat}, the algorithm yields
\[
{\boldsymbol P}{\boldsymbol M}_{\tilde{\boldsymbol y}}{\boldsymbol P}^\top=
{\boldsymbol P}{\boldsymbol V}^\top{\boldsymbol \Lambda}{\boldsymbol V}{\boldsymbol P}^\top=
\widetilde{\boldsymbol V}^\top{\boldsymbol \Lambda}\widetilde{\boldsymbol V}
={\boldsymbol L}{\boldsymbol L}^\top
\]
with \(\widetilde{\boldsymbol V}\isdef {\boldsymbol V}{\boldsymbol P}^\top\).
The above variant of the pivoted Cholesky algorithm is tailored to
the extraction algorithm from \cite[Section 4.3]{Lasserre}, as  the choice
of pivots is restricted to the principal block of size
\(m_q\times m_q\). Note that this amounts to a total pivoting
within this block.
We remark that ${\boldsymbol L}$ and $\widetilde{\boldsymbol V}^\top$ have the same span,
and \({\boldsymbol L}\) can be
permuted such that is upper triangular with non-vanishing diagonal
entries. In particular, \({\boldsymbol L}\) exhibits a column echelon form,
where the upper block is an identity matrix, i.e.\
\[
\widetilde{\boldsymbol L}=\begin{bmatrix}
1 & & \\
& \ddots & \\
& & 1\\
\star &\cdots &\star\\
\vdots & \ddots &\vdots\\
\star &\cdots &\star
\end{bmatrix}.
\]
In complete analogy to \cite{Lasserre}, there exists now a set of monomials
\({\boldsymbol x}^{\boldsymbol\alpha_j}\), \(j=1,\ldots,r\), where the indices \({\boldsymbol\alpha_j}\)
correspond to the \(r\) indices selected by the pivoted Cholesky decomposition
in their order of selection. In particular, there holds now
\begin{equation}\label{eq:extractIdent}
{\boldsymbol P}{\boldsymbol\tau}^\top({\boldsymbol\xi}_j)=\widetilde{\boldsymbol L}{\boldsymbol w}({\boldsymbol\xi}_j)\quad\text{for }j=1,\ldots,r,
\end{equation}
where \({\boldsymbol w}({\boldsymbol x})\isdef[{\boldsymbol x}^{\boldsymbol\alpha_1},\ldots,{\boldsymbol x}^{\boldsymbol\alpha_r}]^\top\).
 
Next, as the pivots are only selected in the upper \(m_q\times m_q\) block,
for each index \({\boldsymbol\alpha_j}\), the index \({\boldsymbol\alpha_j}+{\boldsymbol e}_i\), \(i=1,\ldots,d\)
is also contained in \(\boldsymbol\tau\). In view of \eqref{eq:extractIdent},
forming for \(i=1,\ldots, d\) the submatrices ${\boldsymbol N}_i$ containing the rows
of \(\widetilde{\boldsymbol L}\) corresponding to the indices \({\boldsymbol\alpha_j}+{\boldsymbol e}_i\),
leads to  \(d\) eigenvalue problems
\[
{\boldsymbol N}_i{\boldsymbol w}({\boldsymbol x})=x_i{\boldsymbol w}({\boldsymbol x})\quad\text{for }i=1,\ldots, d.
\] 
The sought scenarios \(\boldsymbol\xi_i\) are now the joint eigenvalues of these problems, i.e.,
\[
{\boldsymbol N}_i{\boldsymbol w}({\boldsymbol\xi}_j)=\xi_{j,i}{\boldsymbol w}({\boldsymbol\xi}_j)\quad\text{for }i=1,\ldots, d,\ j=1,\ldots,r.
\]
As \({\boldsymbol w}({\boldsymbol\xi}_j)\) for
\(j=1,\ldots,r\) are the joint eigenvectors of all
multiplication matrices \({\boldsymbol N}_i\), they may now be computed from a random
convex combination of $\boldsymbol N_i$,
\[
{\boldsymbol N}=\sum_{i=1}^d\rho_i{\boldsymbol N}_i.
\]
Finally, letting \({\boldsymbol N}={\boldsymbol Q}{\boldsymbol T}{\boldsymbol Q}^\top\) denote the ordered Schur decomposition of \({\boldsymbol N}\),
we  arrive at
\[
\xi_{j}(i)={\boldsymbol q}_j^\top{\boldsymbol N}_i{\boldsymbol q}_j\quad\text{for }i=1,\ldots, d,\ j=1,\ldots,r,
\]
where \({\boldsymbol q}_j\) is the \(j\)-th column of \({\boldsymbol Q}\).
If Algorithm~\ref{algo:pivChol_flat} is run with \(\varepsilon=0\), we retrieve the Vandermonde
form of the flat extension \({\boldsymbol M}_{\tilde{\boldsymbol y}}\) with the preceding procedure. Algorithm~\ref{alg:compllll}
summarizes the computational steps.

\begin{algorithm}
\caption{Lasserre's extraction algorithm specialized to pivoted Cholesky decomposition}
\label{alg:compllll} 
\begin{flushleft}
\begin{tabular}{ll}
\textbf{input:}  & symmetric and positive semi-definite moment matrix ${\boldsymbol M_{\boldsymbol y}}\in\mathbb{R}^{m_q\times m_q}$, \\
& rank \(\boldsymbol M_{\boldsymbol y}=r\)\\
\textbf{output:} &  \(r\) scenarios \(\Xi \isdef \big\{\boldsymbol \xi_1,\cdots,\boldsymbol\xi_r\big\}\)
\end{tabular}
\end{flushleft}
%==================================================================================
\begin{algorithmic}[1]
\State Perform pivoted Cholesky decomposition to obtain
\begin{equation*}
    \boldsymbol P \boldsymbol M_{\boldsymbol y} \boldsymbol P^\top = \boldsymbol P\boldsymbol V^\top \boldsymbol \Lambda \boldsymbol V \boldsymbol P^\top  = \widetilde{\boldsymbol V}^{\top} \boldsymbol \Lambda \widetilde{\boldsymbol V} = \boldsymbol L \boldsymbol L^{\top}
\end{equation*}
\State Reduce $\boldsymbol L$ to an echelon form $\widetilde{\boldsymbol L}$. 
\State Extract from $\widetilde{\boldsymbol L}$ the multiplication matrices $\boldsymbol N_{i}, i = 1, \cdots , d$.
\State Compute $\boldsymbol N \isdef \sum_{i=1}^{d} \rho_i \boldsymbol N_i$ with random convex combination.
\State Compute the Schur decomposition $\boldsymbol N = \boldsymbol Q \boldsymbol T \boldsymbol Q^{\top}$ with $\boldsymbol Q = \big[\boldsymbol q_1 \ldots \boldsymbol q_r\big]$.
\State Extract $\boldsymbol \xi_{j}(i) =  \boldsymbol q_{j}^{\top} \boldsymbol N_{i} \boldsymbol q_{j}, i = 1, \ldots , d, \hspace{2pt} j = 1, \ldots , r$.
\end{algorithmic}
\end{algorithm}

For a given Vandermonde decomposition 
${\boldsymbol V}^\top(\boldsymbol\xi_1,\ldots,\boldsymbol\xi_r){\boldsymbol \Lambda}
{\boldsymbol V}(\boldsymbol\xi_1,\ldots,\boldsymbol\xi_r)$ with scenarios
 $\boldsymbol\xi_1,\ldots,\boldsymbol\xi_r$, it remains to compute their probabilities
 $\lambda_1,\ldots,\lambda_r$ in accordance with the input moment matrix
 ${\boldsymbol M}_{\boldsymbol y}$.
%To this end, we employ the following algorithm.
%\begin{algorithm}[htb]\caption{Least-squares weights}\label{algo:leastsquares}
%\begin{enumerate}
% \item Calculate the generalized inverse (for instance using SVD) $\boldsymbol V ^\dagger$ of $\boldsymbol M_{\boldsymbol y}$
% \item Calculate $\boldsymbol m_y\isdef \diag ((V ^{\dagger })^\top\boldsymbol M_{\boldsymbol y}  V ^{\dagger})$
% \item With $\boldsymbol p \isdef \diag \boldsymbol \Lambda$
% \begin{align*}
%  \underset{\boldsymbol p \in \Rbb ^{r}_{+}}{\text{ minimize }} & \|\boldsymbol m_y -\boldsymbol p \|_2^2 \\
%  \text{subject to } & \boldsymbol 1^\top \boldsymbol p = 1
% \end{align*}
%\end{enumerate}
%\end{algorithm} 

\section{Greedy maximum-volume scenarios}
A quasi-Monte Carlo method to construct good quadrature rules, 
with a small number of nodes, to approximate integrals is the so-called Approximate Fekete points (AFP), cf.\
\cite{BosSDeMarchiSommarivaVianello, SOMMARIVA20091324, bittante}. The computation of these points, which give us the scenarios from \eqref{eq:unconstrained_optimization} is done
via a greedy selection of the maximum volume submatrix of the transpose of the Vandermonde matrix. It turns out to be numerically equivalent to
a column-pivoted QR factorization of $\boldsymbol V^\top$, cp.\
\cite{bittante,BSV10,BosSDeMarchiSommarivaVianello,GVL13,SOMMARIVA20091324}\ which tries to give a computational solution to the basis choice problem.  The procedure is summarized in Algorithm~\ref{algo:maxvol}. 
\begin{algorithm}\caption{Maximum volume scenarios (\cite{BosSDeMarchiSommarivaVianello}) }
\label{algo:maxvol}\ \\
\begin{flushleft}
\begin{tabular}{ll}
\textbf{input:}  & matrix \(\boldsymbol Q \in \Rbb^{N \times m}\) \\
\textbf{output:} & index set \(\operatorname{ind}\) corresponding to the sparse scenarios
\end{tabular} 
\end{flushleft}
%=======================================
\begin{algorithmic}[1]
\State Initialization: set \(\boldsymbol W \isdef \boldsymbol Q^\top, \, \boldsymbol w_i \isdef \|\boldsymbol W_i\|_2^2\) for \(i \in \{1,\ldots,N\}, \, \operatorname{ind} \isdef [\,]\)
\State \textbf{for} $k = 1,\ldots,m$ (greedy algorithm for maximum volume submatrix)
\smallskip
\State\StateIndent set \(i_k \isdef \operatorname{arg}\max \{ \boldsymbol w_i : i \notin \operatorname{ind}\}\)
\State\StateIndent set \(\operatorname{ind} \isdef [\operatorname{ind}, \, i_k]\)
\smallskip
\State\StateIndent set \(\boldsymbol w_i \isdef \|\boldsymbol W_i\|_2^2 - \dfrac{(\boldsymbol W_i^\top \boldsymbol W_{i_k})^2}{\|\boldsymbol W_{i_k}\|_2^2}\) for \(i \notin \operatorname{ind}\)
\State \textbf{end}
\end{algorithmic}
\end{algorithm}
The core of the algorithm is given by lines 3-5 and can be efficiently implemented by the \textit{QR factorization with column pivoting}, see \cite{ENGLER19977}. We remark that we can take the number of iterations to be less than $m$ in line 2 of Algorithm \eqref{algo:maxvol} for a prior estimated sparsity level of the number of scenarios.

\section{Greedy thresholding method}\label{sec:gradient_methods}
We put herein an iterative greedy method that is used to solve problems of the form \eqref{eq:modified_unconstrained_optimization}. The algorithm called the hard thresholding pursuit algorithm (HTP), is popular in compressive sensing literature, see \cite{foucart2013mathematical, HTP}. It performs sparse recovery in a stable and robust manner, and in particular, it is used to obtain sparse solutions to linear underdetermined systems. We apply a variant of the HTP, called the graded hard thresholding pursuit (GHTP), cp. \cite{GHTP}, where the size of the index set increases with the number of iterations. We put the steps of GHTP in Algorithm~\ref{algo:GHTP}.
\begin{algorithm}
\caption{Graded hard thresholding pursuit (\cite{GHTP})}
\label{algo:GHTP}
\begin{flushleft}
\begin{tabular}{ll}
\textbf{input:}  & matrix ${\boldsymbol Q}\in\mathbb{R}^{N \times m}$, vector
\(\widetilde{{\boldsymbol y}} \in \Rbb^{m} \), tolerance \(\varepsilon > 0\),
\\ & and maximum number of iterations $J$ \\
\textbf{output:} & index set $\text{ind}$ corresponding to a sparse solution of \eqref{eq:modified_unconstrained_optimization}
\end{tabular}
\end{flushleft}
%%%%%%%%%%%%%%%%%%%%%%%%%%%%%%%%%%%%%%%%%%%%%%%%%%%%%%%%%%%%%%%%%%%%%%%%
\begin{algorithmic}[1]
\State Initialization: set $S^{0} \isdef \varnothing$, $\boldsymbol w^0 \isdef \boldsymbol 0, \text{ind} \isdef [\,]$
\smallskip
\State \textbf{while} \(\text{err} > \varepsilon\,\) \textbf{and} \(\, k<J\)
\smallskip
\State\StateIndent set \(S^{k} \isdef\) index set of $k$ largest absolute entries of \(\boldsymbol w^{k-1} - \boldsymbol Q(\boldsymbol Q^\top \boldsymbol w^{k-1} - \widetilde{\boldsymbol y})\)
\State\StateIndent set \(\boldsymbol w^{k} \isdef \argmin\big\{\|\boldsymbol Q^\top \boldsymbol z - \widetilde{\boldsymbol y}\|_2, \supp({\boldsymbol z}) \subseteq S^{k}\big\}\)
\State\StateIndent set \(\text{err} \isdef \|\boldsymbol Q^\top \boldsymbol w^k - \widetilde{\boldsymbol y}\|_2\)
\State\StateIndent set \(k\isdef k+1\)
\State \textbf{end}
\smallskip
\State \( \text{ind} = \textit{indices of non-zero components of $\boldsymbol w^k$}\)
\end{algorithmic}
\end{algorithm}   
\end{comment}
